# Supplementary material for: GPTNT: Benchmarking Real-Time Collaboration Between Multimodal Agents on Keep Talking And Nobody Explodes
Source: arXiv:2606.28514 source file (2026-09-04)
Supplement: Supplementary file 1 [file action_space.tex]

\levelstay{Action Space}\label{app:action_space}

Every model output must contain a single action expressed as a JSON object, wrapped in an \texttt{<action>} XML tag. Within this, all actions share the same JSON structure:

\vspace{-15pt}
\begin{minted}[frame=lines,framesep=10pt,ignorelexererrors=true]{json}
{"result": {"kind": "...", "data": {...}}}
\end{minted}
\vspace{-10pt}

The \texttt{kind} field identifies the action category, and the \texttt{data} field carries the kind-specific arguments. We define three top-level kinds:
\begin{enumerate}
    \item \texttt{interact\_game}: all manipulation of game elements
    \item \texttt{send\_message}: send a text string to the other player
    \item \texttt{do\_nothing}: choose to skip their turn and do nothing
\end{enumerate}

The schema is both role- and condition-specific. The Defuser receives a schema covering all three kinds. The Expert receives a strict subset that does \textit{not} include \texttt{interact\_game}. Additionally, \texttt{send\_message} is only included when a partner is present in the game---e.g., when models must use parametric knowledge (\cref{sec:e2-parametric-knowledge}) or perform without the Expert (\cref{sec:solo-player})---to prevent models from dispatching outputs to non-existent recipients.

\subimportlevel{action_space}{do_nothing}{1}
\subimportlevel{action_space}{message}{1}
\subimportlevel{action_space}{navigation}{1}
\subimportlevel{action_space}{interact}{1}
