# Supplementary material for: GPTNT: Benchmarking Real-Time Collaboration Between Multimodal Agents on Keep Talking And Nobody Explodes
Source: arXiv:2606.28514 source file (2026-09-04)
Supplement: Supplementary file 2 [file do_nothing.tex]

\levelstay{Do Nothing.}

Both the Defuser and Expert can provide a \texttt{do\_nothing} action on any turn:

\vspace{-15pt}
\begin{minted}{json}
{"result": {"kind": "do_nothing", "data": {}}}
\end{minted}
\vspace{-10pt}

This is a first-class schema action carrying no penalty. In using it, the model signals that it has decided that acting would be premature, unnecessary, or counterproductive given the current game state.

\paragraph{Waiting for the other player.}
In asynchronous mode the game loop does not pause between turns, so a player will often complete a forward pass while the other is mid-sequence. Rather than forcing noisy output, either player can simply wait---the Expert when the Defuser is executing a sequence requiring no input, and the Defuser when awaiting further guidance from the Expert.

\paragraph{Holding the button.}
\texttt{do\_nothing} is the \textit{only} valid action during a \texttt{hold} sequence in the \button module. As the Defuser must output \texttt{release} once a specific target digit appears on the countdown timer strip, they must wait for however many turns are required.

\paragraph{Observing timed blink sequences.}
For \morsecode and \simonsays, the full 16-frame buffer is transmitted each forward pass. Despite our best attempts, if the observation window is misaligned with the blink period, the buffer may not contain a complete sequence. The correct response is to emit \texttt{do\_nothing} and re-observe on the following turn---mirroring the strategy a human player would use under the same conditions.\looseness=-1
