# Supplementary material for: GPTNT: Benchmarking Real-Time Collaboration Between Multimodal Agents on Keep Talking And Nobody Explodes
Source: arXiv:2606.28514 source file (2026-09-04)
Supplement: Supplementary file 3 [file interact.tex]

\begin{table}[tbh]
\centering

\footnotesize
\caption{Interaction actions available to the Defuser with \texttt{interact\_game}.}
\label{tab:interaction_actions}
\begin{tabular}{@{}lll@{}}
\toprule
Sub-action   & Location required & Description \\
\midrule
\texttt{click\_release} & Yes & Press and immediately release; standard for most elements \\
\texttt{hold}           & Yes & Initiate a sustained press at the specified location \\
\texttt{release}        & No  & Terminate an active \texttt{hold} \\
\bottomrule
\end{tabular}
\end{table}

\levelstay{Interaction Actions}\label{app:action_space:interactions}

Interaction actions (\cref{tab:interaction_actions}) operate on a specific screen location and require a \texttt{location} argument. The \gptnt benchmark supports multiple coordinate systems to accommodate different models; all are normalised to relative coordinates internally before being dispatched to the game.

\paragraph{Coordinate systems.}
Three systems are supported:

\begin{itemize}[leftmargin=*]
  \item \textbf{Absolute:} integer pixel values in \([0, x_{\max}] \times [0, y_{\max}]\), with \((0,0)\) at the top-left corner.
  \item \textbf{Scaled:} integer values in \([0, 1000]\) on each axis, independent of render resolution.
  \item \textbf{Relative:} floating-point values in \([0, 1]\) on each axis.
\end{itemize}

\paragraph{Set-of-Marks.}
For models that do not support coordinate output, elements can be targeted using SoM labels. The system resolves a label to the centroid of the corresponding element's bounding region in relative coordinates. An example output using a SoM label:

\needspace{12\baselineskip}
\vspace{-15pt}
\begin{minted}{json}
{
  "result": {
    "kind": "interact_game",
    "data": {
      "action": "click_release",
      "location": "B"
    }
  }
}
\end{minted}
\vspace{-10pt}
