# Supplementary material for: GPTNT: Benchmarking Real-Time Collaboration Between Multimodal Agents on Keep Talking And Nobody Explodes
Source: arXiv:2606.28514 source file (2026-09-04)
Supplement: Supplementary file 4 [file navigation.tex]

\levelstay{Navigation Actions}\label{app:action_space:navigation}

Navigation actions are issued under the \texttt{interact\_game} kind and solely move the bomb to show different perspectives. Therefore, they require no location argument.

\needspace{12\baselineskip}
\vspace{-15pt}
\begin{minted}{json}
{
  "result": {
    "kind": "interact_game",
    "data": {
      "action": "rotate_left"
    }
  }
}
\end{minted}
\vspace{-10pt}

In \cref{tab:navigation_actions}, we outline the various navigation actions and how the bomb is rotated. Note that models must explicitly choose to zoom out to then be able to zoom into another module. However, if a model performs a navigation action while zoomed into a module, we automatically zoom out and then perform that action.

\begin{table}[htb]
\centering
\footnotesize

\caption{Navigation sub-actions available to the Defuser under \texttt{interact\_game}.}
\label{tab:navigation_actions}
\begin{tabular}{@{}lll@{}}
\toprule
Sub-action & Effect & Face exposed \\
\midrule
\texttt{rotate\_left}  & Rotate the bomb 90° counter-clockwise (yaw) & Adjacent side face \\
\texttt{rotate\_right} & Rotate the bomb 90° clockwise (yaw)        & Adjacent side face \\
\texttt{flip}          & Rotate the bomb 180°                        & Opposite side face \\
\texttt{roll\_up}      & Roll the bomb upward 90°                    & Bottom face        \\
\texttt{roll\_down}    & Roll the bomb downward 90°                  & Top face           \\
\texttt{zoom\_out}     & Exit the current module zoom                & Current face (un-zoomed) \\
\bottomrule
\end{tabular}

\end{table}
