# Supplementary material for: GPTNT: Benchmarking Real-Time Collaboration Between Multimodal Agents on Keep Talking And Nobody Explodes
Source: arXiv:2606.28514 source file (2026-09-04)
Supplement: Supplementary file 5 [file do_models_know_ktane.tex]

\levelstay{KTANE Is in the Common Crawl}\label{app:how-do-you-do}

Models are trained on vast corpora of internet data, typically including the Common Crawl (CC) dataset. We establish that the URL hosting the manual\footnote{\url{www.bombmanual.com}} was first captured in CC-MAIN-2016-22 as a result of the May 2016 crawl, a few months after the release of the game in October 2015. This is significantly earlier than all the knowledge cut-off points for all models tested (see \cref{app:models} for more details). However, we cannot say for certain that all models have been trained on this portion of Common Crawl.

\levelstay{Models Can Parrot the Manual from Memory}

To verify which models have been exposed to \ktane during training, we conduct a short preliminary experiment.
For this, we take each module and ask the following question (filling in the placeholder with the name):\looseness=-1
\begin{quote}
    \textit{How do you solve the \textcolor{ooftblue}{\{module\}} module in KTANE?}
\end{quote}
We compare each result to see whether models directly mention \ktane by performing a string-match against either \textit{``Keep Talking and Nobody Explodes''} or \textit{``KTANE''}. In addition, a domain Expert (one of the authors) reviews the outputs to check whether they are plausible-sounding---i.e., without further inspection, does it appear that the model knows what to do.

\cref{app:tab:how-do-you-do} (left) demonstrates that every model knows what \ktane is and can provide plausible details for how to solve every module.
In addition, \cref{app:tab:how-do-you-do} (right) shows that only InternVL does not reliably associate these module names with \ktane without an explicit prompt.
Importantly, this is not necessarily a weakness: the benchmark is designed so that difficulty primarily arises from the collaboration, and not from prior knowledge of the game.

\begin{table}[tbh]
\centering
\footnotesize
\setlength{\tabcolsep}{2pt}

\caption{
String-match results checking whether each model references \textit{Keep Talking and Nobody Explodes} (or \textit{KTANE}) when asked \textit{``How do you solve the \{module\} module [in KTANE]?''}, with and without explicitly naming the game in the prompt.}
\label{app:tab:how-do-you-do}
\begin{tabularx}{\textwidth}{@{}X *{11}{c} p{0cm} *{11}{c}@{}}
    \toprule
    & \multicolumn{11}{c}{With KTANE mentioned}
    && \multicolumn{11}{c}{Without KTANE mentioned} \\
    \cmidrule(r){2-12}\cmidrule(l){14-24}

      & {\wires*}
      & {\button*}
      & {\keypad*}
      & {\simonsays*}
      & {\whosonfirst*}
      & {\memory*}
      & {\maze*}
      & {\morsecode*}
      & {\complicatedwires*}
      & {\wiresequence*}
      & {\passwords*}
      && {\wires*}
      & {\button*}
      & {\keypad*}
      & {\simonsays*}
      & {\whosonfirst*}
      & {\memory*}
      & {\maze*}
      & {\morsecode*}
      & {\complicatedwires*}
      & {\wiresequence*}
      & {\passwords*} \\
    \midrule
    \claude*~Sonnet 4.6
      & \success* & \success* & \success* & \success* & \success* & \success* & \success* & \success* & \success* & \success* & \success
      && \success* & \success* & \success* & \success* & \success* & \success* & \success* & \success* & \success* & \success* & \success* \\
    \gemini*~Gemini 3 Flash
      & \success* & \success* & \success* & \success* & \success* & \success* & \success* & \success* & \success* & \success* & \success
      && \success* & \success* & \success* & \success* & \success* & \success* & \success* & \success* & \success* & \success* & \success* \\
    \openai*~GPT-5.2
      & \success* & \success* & \success* & \success* & \success* & \success* & \success* & \success* & \success* & \success* & \success
      && \success* & \success* & \success* & \success* & \success* & \success* & \success* & \success* & \success* & \success* & \success* \\
    \internvl*~InternVL 3.5 (38B)
      & \success* & \success* & \success* & \success* & \success* & \success* & \success* & \success* & \success* & \success* & \success
      && \strikeout* & \success* & \strikeout* & \success* & \strikeout* & \strikeout* & \success* & \strikeout* & \success* & \strikeout* & \strikeout* \\
    \qwen*~Qwen3.5 (27B)
      & \success* & \success* & \success* & \success* & \success* & \success* & \success* & \success* & \success* & \success* & \success
      && \success* & \success* & \success* & \success* & \success* & \success* & \success* & \success* & \success* & \success* & \success* \\
    \bottomrule
  \end{tabularx}
\end{table}

\FloatBarrier
\levelstay{Models Refer to Their Own Parametric Knowledge}\label{app:example:model-referring-to-param}

We see evidence in Defusers' messages and thoughts that they try to leverage existing knowledge of \ktane's rules. For example, \cref{fig:sonnet-param-knowledge} shows how in a single module \keypad game played with Sonnet as the Defuser and GPT as the Expert,\footnote{\texttt{single\_module\_sync\_Keypad\_561\_(defuser=claude46--expert=gpt5)\_attempt1}} Sonnet, the model \textit{without} access to the manual, tries to justify why the Expert's answers are different from their expectations.

\begin{figure}[ht]
    \centering
    \includegraphics[width=\linewidth]{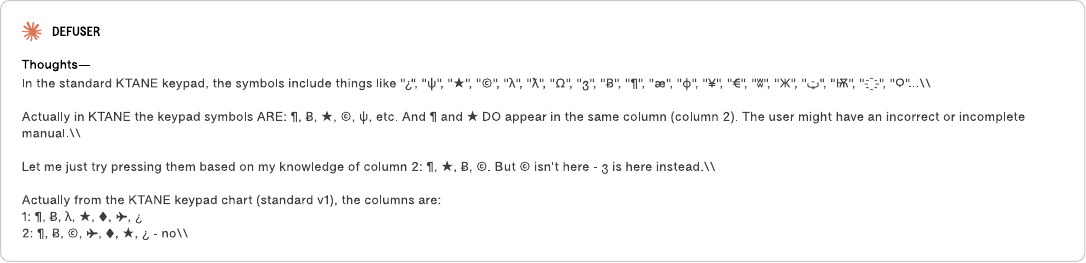}
    \caption{Example of Sonnet recalling the manual from its parametric knowledge.}
    \label{fig:sonnet-param-knowledge}
\end{figure}
