# Supplementary material for: GPTNT: Benchmarking Real-Time Collaboration Between Multimodal Agents on Keep Talking And Nobody Explodes
Source: arXiv:2606.28514 source file (2026-09-04)
Supplement: Supplementary file 6 [file e1-behaviour-profile.tex]

\levelstay{Behavioural Signatures of Failed Games by Model}\label{app:extra:behaviour_signatures}
\cref{fig:behaviour} demonstrates that, on average, the behavioural patterns of the Defuser and Expert players in failed games differ structurally depending on whether the players run out of time or cause too many strikes. In \cref{tab:e1-behavior} we break this down further to reveal how different models can succeed, strike out, or time out with different behavioural signatures. For instance, InternVL's behavioural signature when playing the Defuser suggests a tendency to wait or message the other player over exploring or interacting with the bomb. This skew is most pronounced on successful games, indicating that there is no single strategy to succeed. Similarly, in comparison with other models, Gemini tends to wait significantly less than any other model as the Expert, which can be observed across game outcomes, hinting at model-specific idiosyncrasies that do not affect models' chances to succeed.

\begin{table}[tbh]\centering\footnotesize
\begin{threeparttable}
\caption{Distribution of action types (\% of game steps) by model, role and game outcome played by all possible model pairings on single-module missions in \textit{synchronous} mode. Both players can either wait or send a message (Msg). The Defuser can additionally navigate (Nav) or interact with objects (Int).}
\label{tab:e1-behavior}
\begin{tabular}{@{}p{1.0mm} l c c c c c c c c c c c c @{}}\toprule
 & &  \multicolumn{4}{c}{\success* Solved} & \multicolumn{4}{c}{\strikeout* Strikeout} & \multicolumn{4}{c}{\timeout* Timeout}\\ \cmidrule(lr){3-6} \cmidrule(lr){7-10} \cmidrule(lr){11-14}
& & {\scriptsize Wait} & {\scriptsize Msg} & {\scriptsize Nav} & {\scriptsize Int} & {\scriptsize Wait} & {\scriptsize Msg} & {\scriptsize Nav} & {\scriptsize Int} & {\scriptsize Wait} & {\scriptsize Msg} & {\scriptsize Nav} & {\scriptsize Int}\\ \midrule
\multirow{5}{*}{\rotatebox[origin=c]{90}{\textbf{\textls[25]{Defuser}}}} & \claude*~Sonnet 4.6 & 3.9 & 22.0 & 26.9 & 47.3 & 4.8 & 22.9 & 24.0 & 48.3 & 8.1 & 13.0 & 50.1 & 28.8\\
  & \gemini*~Gemini 3 Flash & 2.5 & 30.9 & 21.7 & 44.8 & 1.3 & 33.7 & 18.2 & 46.7 & 0.9 & 8.6 & 71.1 & 19.5\\
  & \openai*~GPT-5.2 & 5.0 & 31.8 & 15.3 & 47.8 & 4.8 & 39.5 & 12.2 & 43.6 & 9.0 & 31.7 & 38.8 & 20.5\\
  & \internvl*~InternVL 3.5 (38B) & 15.3 & 42.8 & 4.8 & 37.1 & 9.2 & 43.6 & 4.9 & 42.3 & 34.8 & 31.7 & 17.6 & 16.0\\
  & \qwen*~Qwen3.5 (27B) & 5.6 & 29.5 & 24.6 & 40.3 & 4.7 & 35.6 & 17.7 & 42.0 & 15.0 & 20.5 & 47.4 & 17.1\\
\midrule[0.1ex]
  & \textit{Average} & 6.5 & 31.4 & 18.7 & 43.5 & 4.9 & 35.1 & 15.4 & 44.6 & 13.6 & 21.1 & 45.0 & 20.4\\
\midrule[0.1ex]
\multirow{5}{*}{\rotatebox[origin=c]{90}{\textbf{\textls[25]{Expert}}}} & \claude*~Sonnet 4.6 & 60.4 & 39.6 & \color{black!40}0.0 & \color{black!40}0.0 & 60.2 & 39.8 & \color{black!40}0.0 & \color{black!40}0.0 & 74.0 & 26.0 & \color{black!40}0.0 & \color{black!40}0.0\\
  & \gemini*~Gemini 3 Flash & 49.1 & 50.9 & \color{black!40}0.0 & \color{black!40}0.0 & 48.9 & 51.1 & \color{black!40}0.0 & \color{black!40}0.0 & 60.4 & 39.6 & \color{black!40}0.0 & \color{black!40}0.0\\
  & \openai*~GPT-5.2 & 61.1 & 38.9 & \color{black!40}0.0 & \color{black!40}0.0 & 59.3 & 40.7 & \color{black!40}0.0 & \color{black!40}0.0 & 72.7 & 27.3 & \color{black!40}0.0 & \color{black!40}0.0\\
  & \internvl*~InternVL 3.5 (38B) & 65.9 & 34.1 & \color{black!40}0.0 & \color{black!40}0.0 & 60.9 & 39.1 & \color{black!40}0.0 & \color{black!40}0.0 & 75.0 & 25.0 & \color{black!40}0.0 & \color{black!40}0.0\\
  & \qwen*~Qwen3.5 (27B) & 61.0 & 39.0 & \color{black!40}0.0 & \color{black!40}0.0 & 57.1 & 42.9 & \color{black!40}0.0 & \color{black!40}0.0 & 68.2 & 31.8 & \color{black!40}0.0 & \color{black!40}0.0\\
\midrule[0.1ex]
  & \textit{Average} & 59.5 & 40.5 & \color{black!40}0.0 & \color{black!40}0.0 & 57.3 & 42.7 & \color{black!40}0.0 & \color{black!40}0.0 & 70.1 & 29.9 & \color{black!40}0.0 & \color{black!40}0.0\\
\bottomrule
\end{tabular}
\end{threeparttable}\end{table}
