# Supplementary material for: GPTNT: Benchmarking Real-Time Collaboration Between Multimodal Agents on Keep Talking And Nobody Explodes
Source: arXiv:2606.28514 source file (2026-09-04)
Supplement: Supplementary file 7 [file keypad-statics.tex]

\levelstay{Describing Keypad Symbols}\label{app:statics:keypad}

The \keypad module requires communicating four of 25 possible symbols that must be pressed in the correct order.
These symbols are visually unfamiliar to English speakers, requiring negotiation of shared meaning.
We devise two offline evaluation settings, each containing 40 samples of keypad modules, to examine how models describe these symbols.
In the multiple-choice setting, models select the description that best matches a given symbol from five choices.
In the open-ended setting, models describe the symbols in free text.
For open-ended responses, we evaluate using a semantic similarity metric against a gold-standard reference set: predicted descriptions are embedded using a Sentence Transformer \citep{reimers-2019-sentence-bert}.\footnote{We use \texttt{sentence-transformers/paraphrase-multilingual-MiniLM-L12-v2}, which has a multilingual vocabulary that includes the rare characters appearing on keypad buttons.}
This tests whether models can produce semantically grounded descriptions of visual elements that lack a common linguistic encoding.\looseness=-1

\begin{table}[tbh]\centering\footnotesize

\caption{Description accuracy for Keypad by question format.}
\label{tab:simulator-vqa-keypad-description}
\begin{threeparttable}

\begin{tabular}{@{}l S[table-format=2.1] S[table-format=2.1] @{}}

\toprule
 & {Multiple-choice} & {Open-ended} \\
\midrule
\claude*~Sonnet 4.6 & 65.0 & 45.0 \\
\gemini*~Gemini 3 Flash & 95.0 & 67.5 \\
\openai*~GPT-5.2 & 65.0 & 42.5 \\
\internvl*~InternVL 3.5 (38B) & 45.0 & 22.5 \\
\qwen*~Qwen3.5 (27B) & 50.0 & 17.5 \\
\midrule[0.1ex]
\textit{Average} & 64.0 & 39.0 \\
\bottomrule
\end{tabular}
\end{threeparttable}
\end{table}

\cref{tab:simulator-vqa-keypad-description} shows the results.
Across all models, performance drops sharply from the multiple-choice to the open-ended setting, indicating that recognising a valid description is considerably easier than generating one---a gap that reflects the open-ended nature of symbol naming rather than any single failure mode.
Similar to other offline evaluations of model capabilities, Gemini stands out as the strongest model in both settings, while Qwen and InternVL cluster together at the lower end.

Inspecting the open-ended descriptions reveals that models use different references for the same symbol, with almost no overlap: for more than half of the symbols, no two models produce the same description.
For instance, the Pashto \textit{tte} letter \pashtote is described as `smiley face' by Gemini and GPT, and `magnet' by Qwen---both considered valid.
Notably, all models converge on a description for exactly one symbol: the hollow star, which every model refers to as `star'.
Our benchmark uses text-based communication, which gives models an advantage over the original setting, which assumes spoken dialogue.
We find that models frequently default to identifying a Unicode character that visually resembles the symbol, rather than describing it in English words.
This converts the communicative challenge into a visual matching problem for the other agent downstream.
We hypothesise that the effects observed here would be exacerbated in a spoken dialogue setting, as this text-specific workaround does not transfer to speech.
