# Supplementary material for: GPTNT: Benchmarking Real-Time Collaboration Between Multimodal Agents on Keep Talking And Nobody Explodes
Source: arXiv:2606.28514 source file (2026-09-04)
Supplement: Supplementary file 8 [file multi-mod-outcome-details.tex]

\levelstay{Supplementary Results: Benchmark Game Outcomes}\label{app:results:multi-outcome-breakdown}

\cref{tab:e7-stats,tab:e5-stats} detail the outcomes from the ten missions using multiple module types introduced in \cref{sec:actual-benchmark}. Models solve, on average, twice as many individual modules when we remove the real-time constraints. Breaking down how modules fail reveals further crucial differences between the two settings: while timeouts dominate in asynchronous mode, models are equally as likely to time out as they are to strike out in synchronous mode. Crucially, we find evidence that models are more likely to time out \textit{before} they even cause their first strike in asynchronous mode.

\begin{table}[tbh]
\centering
\footnotesize

\begin{threeparttable}
\caption{Self-play game outcomes across ten distinct missions in asynchronous mode, where the game is \textit{not paused} while models generate. We examine module completion, strike distribution at timeout, and strikeout timing. Each mission is attempted once (pass@1).}
\label{tab:e7-stats}
\sisetup{table-format=2.1}
\begin{tabular}{@{}l S S S S S S S @{}}
\toprule
 & {} & \multicolumn{4}{c}{\timeout* Timeout} & \multicolumn{2}{c}{\strikeout* Strikeout} \\
\cmidrule(lr){3-6}\cmidrule(l){7-8}
 & {\makecell{\% Modules\\Solved}}
 & {\makecell{\% of\\Failures}}
 & {0 Strikes}
 & {1 Strike}
 & {2 Strikes}
 & {\makecell{\% of\\Failures}}
 & {\makecell{Time\\Elapsed (\%)}} \\
\midrule
\claude*~Sonnet 4.6           & 15.8 & 40.0 & 25.0 & 25.0 & 50.0 & 60.0 & 65.0 \\
\gemini*~Gemini 3 Flash       & 10.0 & 50.0 & 80.0 & \color{black!40}0.0 & 20.0 & 50.0 & 47.0 \\
\openai*~GPT-5.2              & 11.7 & 90.0 & 33.3 & 33.3 & 33.3 & 10.0 & 65.0 \\
\internvl*~InternVL 3.5 (38B) & 3.3  & 70.0 & 57.1 & 14.3 & 28.6 & 30.0 & 18.3 \\
\qwen*~Qwen3.5 (27B)          & 6.7  & 80.0 & 75.0 & 25.0 & \color{black!40}0.0 & 20.0 & 43.1 \\
\midrule
\textit{Average}              & 9.5  & 66.0 & 54.1 & 19.5 & 26.4 & 34.0 & 47.7 \\
\bottomrule
\end{tabular}
\end{threeparttable}
\end{table}

\begin{table}[tbh]
\centering
\footnotesize

\begin{threeparttable}
\caption{Self-play game outcomes across ten distinct missions in \textit{synchronous} mode, where the game \textit{is paused} while models generate. We examine module completion, strike distribution at timeout, and strikeout timing. Each mission is attempted once (pass@1).}
\label{tab:e5-stats}
\sisetup{table-format=2.1}
\begin{tabular}{@{}l S S S S[table-format=3.1] S S S @{}}
\toprule
 &  & \multicolumn{4}{c}{\timeout* Timeout} & \multicolumn{2}{c}{\strikeout* Strikeout} \\
\cmidrule(lr){3-6}\cmidrule(lr){7-8}
 & {\makecell{\% Modules\\Solved}}
 & {\makecell{\% of\\Failures}}
 & {0 Strikes}
 & {1 Strike}
 & {2 Strikes}
 & {\makecell{\% of\\Failures}}
 & {\makecell{Time\\Elapsed (\%)}} \\
\midrule
\claude*~Sonnet 4.6           & 30.0 & 33.3 & 33.3 & \color{black!40}0.0  & 66.7 & 66.7 & 25.3 \\
\gemini*~Gemini 3 Flash       & 15.8 & 60.0 & 50.0 & 33.3                 & 16.7 & 40.0 & 30.7 \\
\openai*~GPT-5.2              & 22.5 & 22.2 & \color{black!40}0.0 & 100.0 & \color{black!40}0.0 & 77.8 & 52.4 \\
\internvl*~InternVL 3.5 (38B) & 11.7 & 70.0 & 28.6 & 14.3                 & 57.1 & 30.0 & 20.4 \\
\qwen*~Qwen3.5 (27B)          & 11.7 & 60.0 & 66.7 & 33.3                 & \color{black!40}0.0 & 40.0 & 28.6 \\
\midrule
\textit{Average}              & 18.3 & 49.1 & 35.7 & 36.2                 & 28.1 & 50.9 & 31.5 \\
\bottomrule
\end{tabular}
\end{threeparttable}
\end{table}

\FloatBarrier
\levelstay{Supplementary Results: Simplified Mission Game Outcomes}\label{app:results:simplified-outcome-breakdown}

\cref{tab:async-single-module-self-play-outcomes,tab:sync-single-module-self-play-outcomes} provide a detailed breakdown of the outcomes from the simplified single-module missions used in \cref{sec:low-level}. Besides a four-fold increase in the number of missions solved, removing the real-time constraints results in a dramatic reduction in timeouts as the primary mode of failure. Where in the asynchronous setting, 84.1\% of missions that fail time out, timeouts only make up 57.4\% of failed missions when we stop the game clock, remaining the dominant mode of failure---albeit by a modest margin.

\begin{table}[tbh]
\centering
\footnotesize

\begin{threeparttable}
\caption{Self-play game outcomes across single-module missions in \textit{asynchronous} mode,
where the game clock \textit{runs continuously} during model generation. We examine mission
completion, strike distribution at timeout, and strikeout timing. Each model attempts
each single-module mission once (pass@1).}
\label{tab:async-single-module-self-play-outcomes}
\setlength{\tabcolsep}{4pt}
\sisetup{table-format=2.1}
\begin{tabular}{@{}l S S[table-format=3.1] S S S S S @{}}
\toprule
 & {\success* Solved} & \multicolumn{4}{c}{\timeout* Timeout} & \multicolumn{2}{c}{\strikeout* Strikeout} \\
\cmidrule(lr){2-2}\cmidrule(lr){3-6}\cmidrule(lr){7-8}
 & {\makecell{\% of\\Missions}}
 & {\makecell{\% of\\Failures}}
 & {0 Strikes}
 & {1 Strike}
 & {2 Strikes}
 & {\makecell{\% of\\Failures}}
 & {\makecell{Time\\Elapsed (\%)}} \\
\midrule
\claude*~Sonnet 4.6           & 12.7 & 84.4 & 50.6 & 32.1 & 17.3 & 15.6 & 71.9 \\
\gemini*~Gemini 3 Flash       & 14.5 & 88.3 & 85.5 & 9.6  & 4.8  & 11.7 & 53.6 \\
\openai*~GPT-5.2              & 8.2  & 92.1 & 65.6 & 24.7 & 9.7  & 7.9  & 79.9 \\
\internvl*~InternVL 3.5 (38B) & 4.5  & 64.8 & 51.5 & 27.9 & 20.6 & 35.2 & 44.8 \\
\qwen*~Qwen3.5 (27B)          & 7.3  & 91.2 & 64.5 & 23.7 & 11.8 & 8.8  & 57.6 \\
\midrule
\textit{Average}              & 9.5  & 84.1 & 63.5 & 23.6 & 12.8 & 15.9 & 61.6 \\
\bottomrule
\end{tabular}
\end{threeparttable}
\end{table}

\begin{table}[tbh]
\centering
\footnotesize

\begin{threeparttable}
\caption{Self-play game outcomes across single-module missions in \textit{synchronous} mode,
where the game clock \textit{pauses} while models generate. We examine mission completion,
strike distribution at timeout, and strikeout timing. Each model attempts each
single-module mission once (pass@1).}
\label{tab:sync-single-module-self-play-outcomes}
\setlength{\tabcolsep}{4pt}
\sisetup{table-format=2.1}
\begin{tabular}{@{}l S S S S S S S @{}}
\toprule
 & {\success* Solved} & \multicolumn{4}{c}{\timeout* Timeout} & \multicolumn{2}{c}{\strikeout* Strikeout} \\
\cmidrule(lr){2-2}\cmidrule(lr){3-6}\cmidrule(lr){7-8}
 & {\makecell{\% of\\Missions}}
 & {\makecell{\% of\\Failures}}
 & {0 Strikes}
 & {1 Strike}
 & {2 Strikes}
 & {\makecell{\% of\\Failures}}
 & {\makecell{Time\\Elapsed (\%)}} \\
\midrule
\claude*~Sonnet 4.6           & 39.1 & 31.3 & 52.4 & 23.8 & 23.8 & 68.7 & 59.2 \\
\gemini*~Gemini 3 Flash       & 20.9 & 64.4 & 80.4 & 5.4  & 14.3 & 35.6 & 49.6 \\
\openai*~GPT-5.2              & 38.2 & 54.4 & 32.4 & 32.4 & 35.1 & 45.6 & 50.9 \\
\internvl*~InternVL 3.5 (38B) & 12.7 & 59.4 & 68.4 & 19.3 & 12.3 & 40.6 & 44.0 \\
\qwen*~Qwen3.5 (27B)          & 10.9 & 77.6 & 65.8 & 23.7 & 10.5 & 22.4 & 55.2 \\
\midrule
\textit{Average}              & 24.4 & 57.4 & 59.9 & 20.9 & 19.2 & 42.6 & 51.8 \\
\bottomrule
\end{tabular}
\end{threeparttable}
\end{table}
