# Supplementary material for: GPTNT: Benchmarking Real-Time Collaboration Between Multimodal Agents on Keep Talking And Nobody Explodes
Source: arXiv:2606.28514 source file (2026-09-04)
Supplement: Supplementary file 9 [file pairwise-communication-rates.tex]

\levelstay{Communication Rates and Verbosity By Pairing}\label{app:extra:communication}

As shown in \cref{tab:e1-msg-pct-self-vs-nonself}, on average, models tend to exchange more messages when paired with a different model in other-play. \cref{fig:verbosity-game-steps} breaks down the proportion of game steps containing a message for each of the 25 possible model pairings. What is more, the role a model plays in a given pairing matters when it comes to the rate of communication the players exhibit while playing a given mission. For instance, when Sonnet is the Defuser and GPT the Expert, 22.4\% of the step budget is spent on communication, while when GPT is the Defuser and Sonnet the Expert, the communication rate increases to 38.1\%. Specifically, the Defuser's communicativeness in self-play defines the floor for the communication rate in other-play.

\begin{figure}[ht]
    \centering
    \includegraphics[width=1\linewidth]{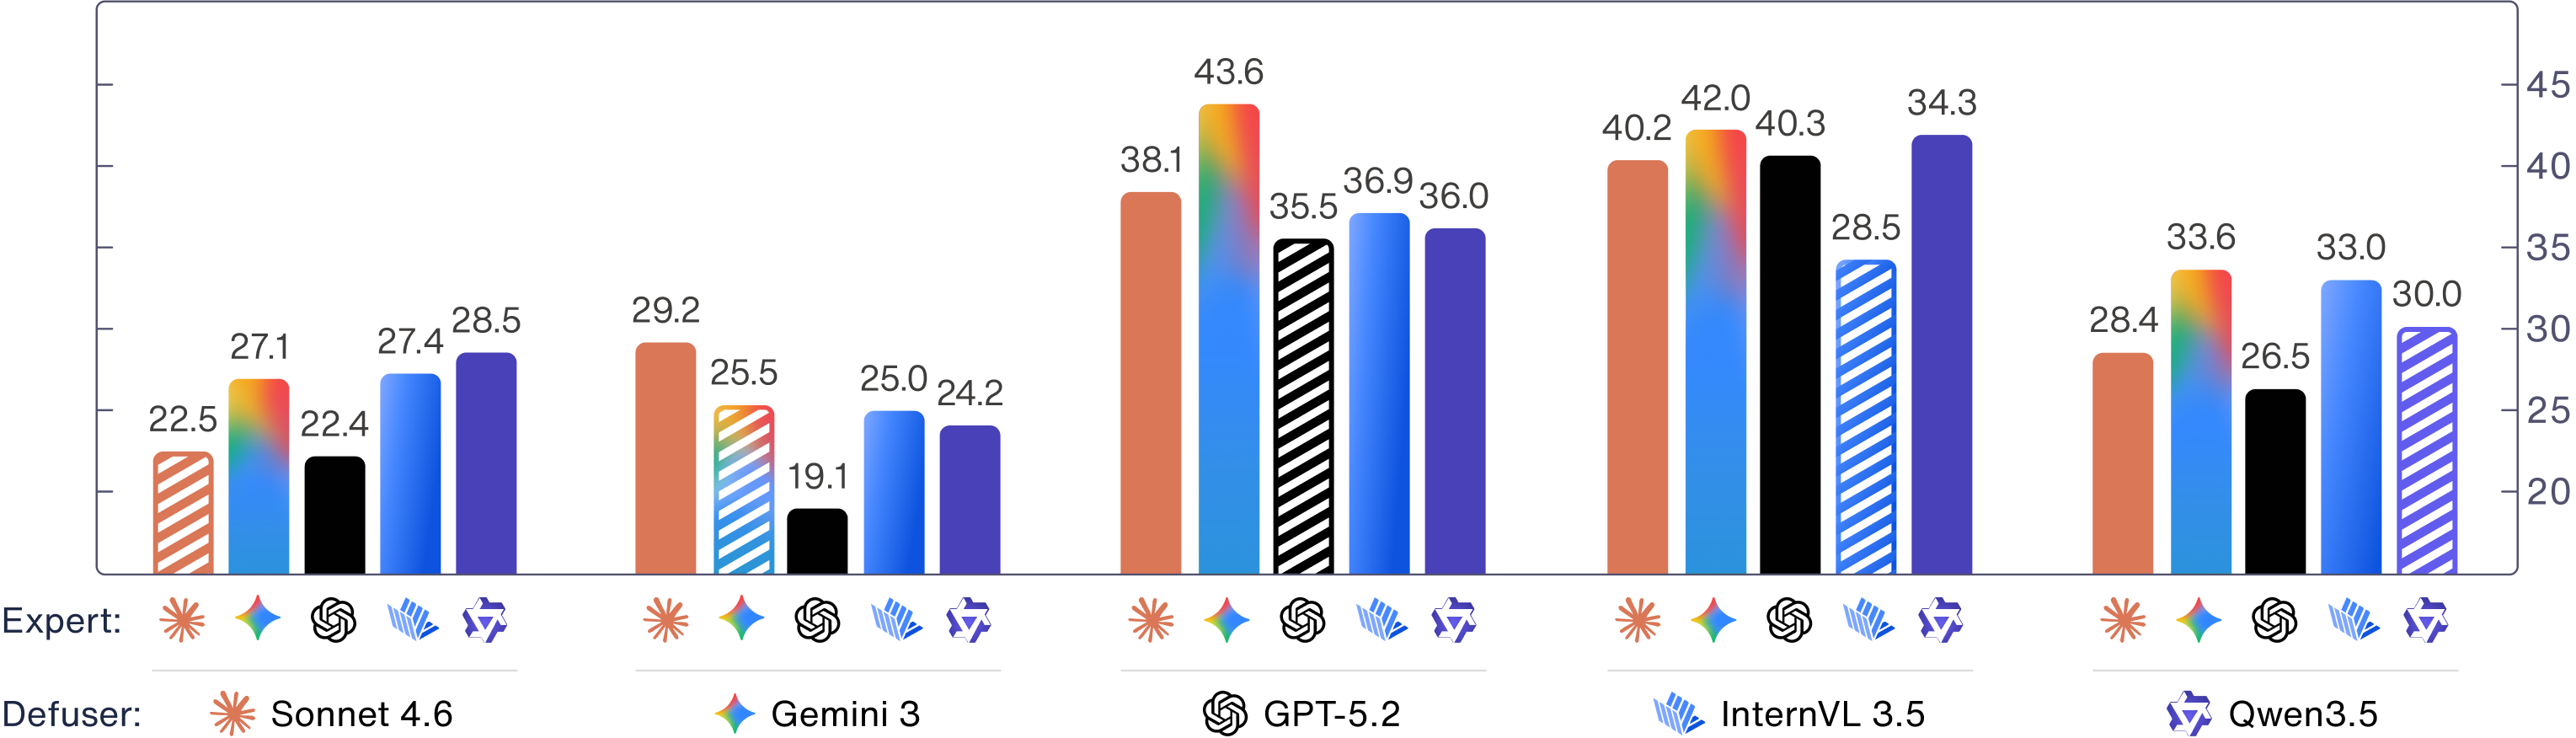}
    \caption{Communication rates for all possible model pairings on the simplified missions with single modules in synchronous mode. Each shows the proportion of game steps in which either player sends a message. Self-play---where both roles are played by an instance of the same model---is highlighted as patterned.}
    \label{fig:verbosity-game-steps}
\end{figure}
