# Supplementary material for: GPTNT: Benchmarking Real-Time Collaboration Between Multimodal Agents on Keep Talking And Nobody Explodes
Source: arXiv:2606.28514 source file (2026-09-04)
Supplement: Supplementary file 10 [file som_vs_coords.tex]

\levelstay{Comparing Set-of-Marks with Coordinates}\label{app:results:som-vs-coords}

Accurate perception alone is not sufficient in \ktane as the Defuser must also act on what it sees.
Given an instruction from the Expert, the Defuser must locate the element and interact with it, grounding language directly to pixels. GUI grounding is an active research area \citep{xie2024osworld,cheng2024seeclick,NEURIPS2025_16130af9}, demonstrating that visual understanding and spatial grounding are separate bottlenecks, and that the interaction protocol can substantially shape performance.
We compare two common paradigms used with VLMs (\cref{fig:statics:simulator-localisation-compare}): \textit{coordinate prediction}, where the model receives a raw screenshot and must output $(x,y)$ coordinates for the target element; and \textit{set-of-marks} (SoM; \citealp{Yang2023SetofMarkPromptingUnleashesa}), where labelled segmentation masks are overlaid on the image and the model selects the correct label.

\begin{figure}[tbh]
\centering
\begin{subfigure}[t]{0.48\textwidth}
\centering
\includegraphics[width=1\linewidth]{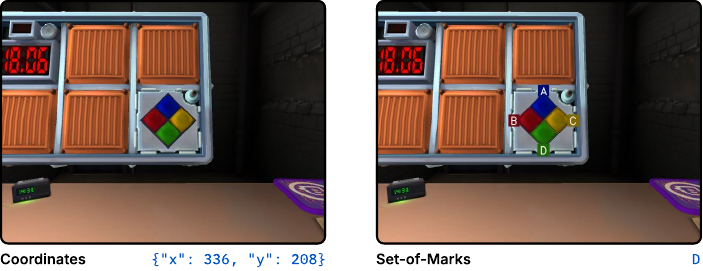}
\caption{Simon Says---\textit{Click on the green button.}}
\end{subfigure}%
\hspace{\fill}%
\begin{subfigure}[t]{0.48\textwidth}
\centering
\includegraphics[width=1\linewidth]{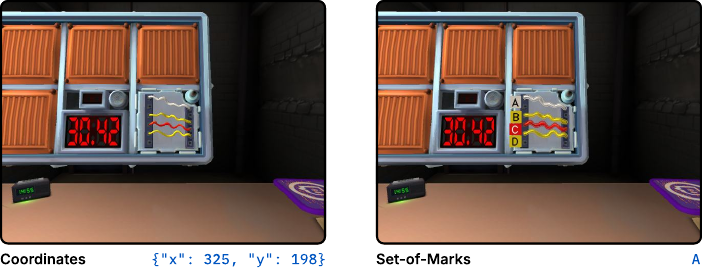}
\caption{Wires---\textit{Click on the first wire.}}
\end{subfigure}%
\caption{Examples from the Simulator Localisation.}
\label{fig:statics:simulator-localisation-compare}
\end{figure}

\begin{table}[tbh]\centering\footnotesize
\begin{threeparttable}
\sisetup{table-format=2.1}
\caption{Accuracy (\%) on Simulator Localisation tasks comparing selecting the correct set-of-marks style location marker with predicting a valid coordinate for actions.}
\label{tab:localization-coordinates-vs-som}
\begin{tabular}{@{}p{1.0mm} l *{11}{S} S @{}}\toprule
 & &  {\wires*} & {\button*} & {\keypad*} & {\simonsays*} & {\whosonfirst*} & {\memory*} & {\maze*} & {\morsecode*} & {\complicatedwires*} & {\wiresequence*} & {\passwords*} & {\textit{Avg.}}\\ \midrule
\parbox[t]{2mm}{\multirow{6}{*}{\rotatebox[origin=c]{90}{\textbf{\textls[25]{Set-of-Marks}}}}} & \claude*~Sonnet 4.6 & 64.3 & \Uline{100.0} & 71.7 & \Uline{100.0} & 77.8 & 95.5 & \Uline{100.0} & \Uline{100.0} & \Uline{74.0} & 60.9 & 76.5 & 80.6 \\
 & \gemini*~Gemini 3 Flash & 64.3 & \Uline{100.0} & \Uline{98.1} & \Uline{100.0} & 53.7 & \Uline{100.0} & \Uline{100.0} & \Uline{100.0} & \Uline{74.0} & \Uline{69.6} & \Uline{97.1} & \Uline{83.9} \\
 & \openai*~GPT-5.2 & \Uline{71.4} & \Uline{100.0} & 81.1 & \Uline{100.0} & 68.5 & 95.5 & \Uline{100.0} & 96.9 & 72.0 & 67.4 & 64.7 & 80.4 \\
 & \internvl*~InternVL 3.5 (38B) & 50.0 & 95.5 & 71.7 & 66.7 & 22.2 & 18.2 & \Uline{100.0} & 65.6 & 58.0 & 37.0 & 23.5 & 53.7 \\
 & \qwen*~Qwen3.5 (27B) & 64.3 & \Uline{100.0} & 73.6 & \Uline{100.0} & 70.4 & \Uline{100.0} & \Uline{100.0} & 96.9 & 64.0 & 58.7 & 58.8 & 76.8 \\
\cmidrule[0.1ex](l){2-14}
 & \textit{Average} & 62.9 & 99.1 & 79.2 & 93.3 & 58.5 & 81.8 & 100.0 & 91.9 & 68.4 & 58.7 & 64.1 & 75.1 \\
\midrule
\parbox[t]{2mm}{\multirow{6}{*}{\rotatebox[origin=c]{90}{\textbf{\textls[25]{Coordinates}}}}} & \claude*~Sonnet 4.6 & 17.9 & 90.9 & 73.6 & 90.5 & 87.0 & 40.9 & 11.4 & 53.1 & 8.0 & 13.0 & 20.6 & 44.6 \\
 & \gemini*~Gemini 3 Flash & 10.7 & 90.9 & 92.5 & 90.5 & \Uline{96.3} & 86.4 & 68.6 & 84.4 & 30.0 & 37.0 & 82.4 & 68.8 \\
 & \openai*~GPT-5.2 & 3.6 & 27.3 & 1.9 & 4.8 & 1.9 & 4.5 & 2.9 & \color{black!40}0.0 & 4.0 & 2.2 & \color{black!40}0.0 & 4.5 \\
 & \internvl*~InternVL 3.5 (38B) & 7.1 & 90.9 & 52.9 & 38.1 & 52.8 & \color{black!40}0.0 & \color{black!40}0.0 & 21.9 & 2.0 & 6.5 & 11.8 & 29.6 \\
 & \qwen*~Qwen3.5 (27B) & 23.1 & \Uline{100.0} & 65.1 & 78.9 & 88.5 & 72.7 & 12.5 & 70.0 & 11.6 & 31.0 & 6.2 & 49.4 \\
\cmidrule[0.1ex](l){2-14}
 & \textit{Average} & 12.5 & 80.0 & 57.2 & 60.6 & 65.3 & 40.9 & 19.1 & 45.9 & 11.1 & 17.9 & 24.2 & 39.4 \\
\bottomrule
\end{tabular}
\end{threeparttable}\end{table}

\cref{tab:localization-coordinates-vs-som} shows that models perform very differently across both paradigms. Under SoM, average performance for the top models clusters between 76.8\% and 83.9\%, suggesting that label selection is reliably within reach. Under coordinate prediction however, those same models span from 4.5\% to 68.6\%. GPT is the clearest illustration of this: 80.4\% under SoM, 4.5\% under coordinates, scoring near-zero for almost every module. This difference indicates a weakness at spatial grounding, as models perform much better when grounding is reduced to label selection.

InternVL's performance suggests an additional failure mode that can exist. Under SoM, it already trails at 53.7\%, but the gap widens sharply on grid-heavy modules: most clearly seen on \memory (18.2\% vs.\ 95.5+\% for other models) and \whosonfirst (22.2\% vs.\ 53.7+\%).
These layouts require models to parse a dense grid and select the correct element within it, indicating that the failure mode is more about layout complexity than the interaction protocol.

Gemini is the only model that carries its SoM performance into coordinates well (83.9\% to 68.6\%).
However, its failure pattern indicates that errors cluster on \wires, \complicatedwires, and \wiresequence---three modules with small interaction targets. Gemini's weaknesses on precision show that it can identify targets but misses a narrow zone. As Gemini is a strong model, it shows that as models get better at coordinate prediction, the details will be a deciding factor.
