# Supplementary material for: GPTNT: Benchmarking Real-Time Collaboration Between Multimodal Agents on Keep Talking And Nobody Explodes
Source: arXiv:2606.28514 source file (2026-09-04)
Supplement: Supplementary file 11 [file resolution.tex]

\levelstay{Image Resolution}

The game modification exports raw RGB24 pixel data from the Unity render buffer on demand. The default capture resolution is 640 × 480 (4:3 aspect ratio), selected as the minimum resolution at which a human player can reliably read all text, labels, and visual indicators present in the game. This serves as the baseline for all models for which context length permits its use.

Two models---Qwen and InternVL---require downsampled resolutions due to context window constraints. At $640 \times 480$, the combined token cost of the Expert's manual and the Defuser's game frames would saturate these models' context windows during tokenisation, leaving insufficient capacity for dialogue history. Qwen therefore receives frames at $448 \times 448$ and InternVL at $504 \times 504$.\footnote{While Qwen has a larger context length and can support the original resolution of observations, we want to make the open-source models comparable, and so we provide images according to the base resolution supported by either model.} All downsampling uses Lanczos filtering. All reduced resolutions are manually verified to remain legible for every module type appearing in the experiments.\looseness=-1

Lower resolution reduces token cost per frame and enables longer retained dialogue histories; higher resolution would improve legibility of fine-grained visual elements---digit labels, wire colours, indicator text---but is cost-prohibitive at the experimental scale reported here.
