# Supplementary material for: GPTNT: Benchmarking Real-Time Collaboration Between Multimodal Agents on Keep Talking And Nobody Explodes
Source: arXiv:2606.28514 source file (2026-09-04)
Supplement: Supplementary file 12 [file set-of-marks.tex]

\levelstay{Set-of-Marks}\label{app:som}

\begin{figure}[tb]
\centering
\begin{subfigure}[t]{0.30\textwidth}
    \centering
    \begin{tikzpicture}
    \clip [rounded corners=5pt] (0,0) rectangle (1\textwidth, 1\textwidth);
    \node[anchor=south west, inner sep=0] at (0,0)
        {\includegraphics[width=1\textwidth]{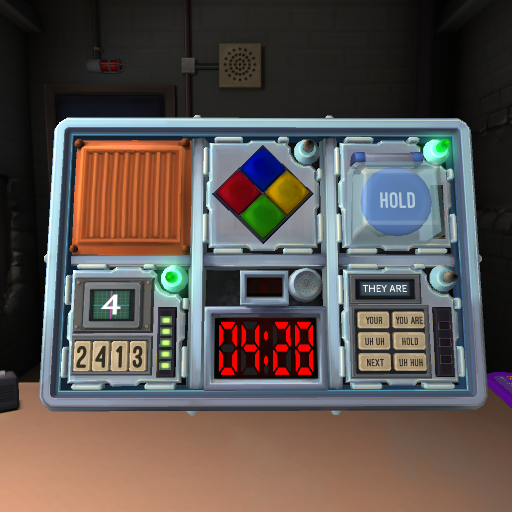}};
    \end{tikzpicture}
    \caption{Original frame}
    \label{fig:som-original}
\end{subfigure}%
\hspace{\fill}
\begin{subfigure}[t]{0.30\textwidth}
    \centering
    \begin{tikzpicture}
    \clip [rounded corners=5pt] (0,0) rectangle (1\textwidth, 1\textwidth);
    \node[anchor=south west, inner sep=0] at (0,0)
        {\includegraphics[width=1\textwidth]{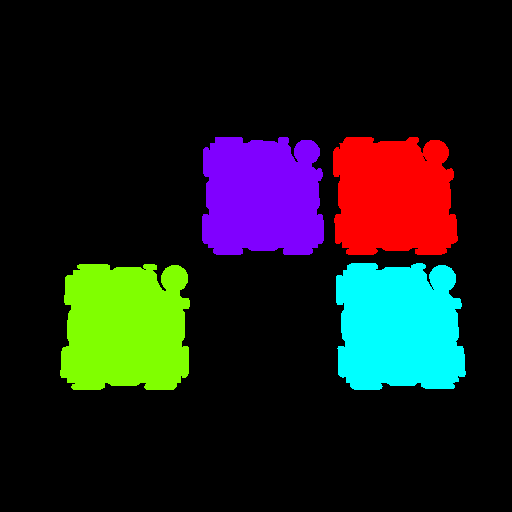}};
    \end{tikzpicture}
    \caption{Segmentation mask}
    \label{fig:som-segm-mask}
\end{subfigure}%
\hspace{\fill}
\begin{subfigure}[t]{0.30\textwidth}
    \centering
    \begin{tikzpicture}
    \clip [rounded corners=5pt] (0,0) rectangle (1\textwidth, 1\textwidth);
    \node[anchor=south west, inner sep=0] at (0,0)
        {\includegraphics[width=1\textwidth]{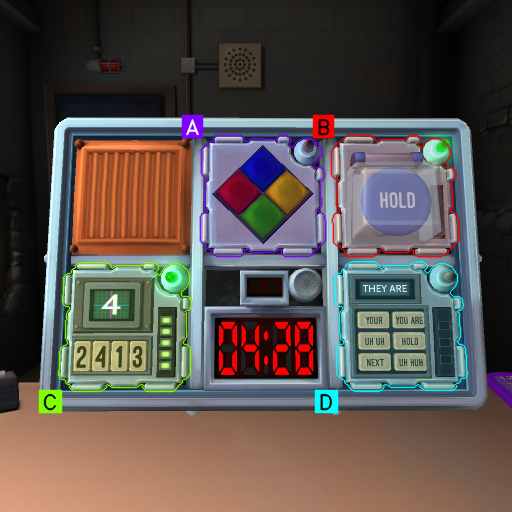}};
    \end{tikzpicture}
    \caption{Image with annotations}
    \label{fig:som-final}
\end{subfigure}%
\caption{Set-of-Marks annotation inputs and outputs. The original frame (a) and segmentation mask (b) are both provided by the environment using our mod. In the segmentation mask, each interactable object is represented by a distinct colour region. Using a heuristic pipeline, we generate the annotated image (c) which combines the previous two images and provide that to the model to facilitate easier identification of interactable elements.}
\label{fig:som-creation}
\end{figure}

Observations given to the Defuser agent include set-of-marks (SoM) annotations \citep{Koh2024VisualWebArenaEvaluatingMultimodal,Yang2023SetofMarkPromptingUnleashesa}, which are used to highlight elements in the current view that are interactable by the agent.
As illustrated by \cref{fig:som-creation}, each interactable element is outlined by a brightly coloured outline, labelled by a label within a box of the same colour. Within any given observation, each interactable element will have a unique label, but labels are not unique across different observations.

\paragraph{Label.}
Letters are used for annotations rather than numbers. As recommended by \citet{Yang2023SetofMarkPromptingUnleashesa} and from preliminary experiments, we find that using numbers leads to mistakes and hallucinations. We attribute this to the presence of numbers on many of the modules, as shown by the \memory module in \cref{fig:som-creation}. Additionally, while the Password module uses letters, using letters for the labels has no noticeable effect on the ability of the model to recognise the text in the display versus the labels. We attribute this to the fact that the letters in the Password module are placed and look distinctly different from the marks.

\paragraph{Position.}
As each bomb module has the same layout, we use heuristics to place the labels such that for any given module, the labels will always be in the same position, relative to their module. Additionally, we ensure that if the number of elements within a module varies, the positioning of labels remains consistent. For example, as illustrated in \cref{fig:sub-wires}, all labels for the Wires module will appear on the left, ordered from top-to-bottom. From preliminary experiments, we find that ordering all labels in a common reading order leads to the most consistent behaviour from models.

\paragraph{Colour.}
As mentioned in \cref{app:game-modules}, some modules rely on colours for their references, meaning that randomly assigning colours is not effective for some modules. This includes the \button, \simonsays and each of the three wire-based modules---\wires, \complicatedwires, and \wiresequence.
In these cases, we match the colour of the mask and label background to the colour of the interactable element. For example, in \simonsays (\cref{fig:simon_som}), the colour for the set-of-marks matches each respective button colour.
This same pattern follows in each wire-based module except for \complicatedwires: as a wire can contain multiple colours, a multi-coloured mask is used in this case, striped with each colour which appears in the wire. An example of this can be observed in \cref{fig:comp-wires-som}.

\begin{figure}[htb]
\centering
\begin{subfigure}[t]{0.2\textwidth}
    \centering
    \begin{tikzpicture}
        \clip [rounded corners=5pt] (0,0) rectangle (0.8\textwidth, 0.8\textwidth);
        \node[anchor=south west, inner sep=0] at (0,0)
            {\includegraphics[width=0.8\textwidth]{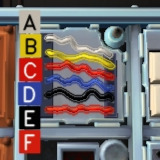}};
    \end{tikzpicture}
    \caption{Wires}
    \label{fig:sub-wires}
\end{subfigure}%
\begin{subfigure}[t]{0.2\textwidth}
    \centering
    \begin{tikzpicture}
        \clip [rounded corners=5pt] (0,0) rectangle (0.8\textwidth, 0.8\textwidth);
        \node[anchor=south west, inner sep=0] at (0,0)
            {\includegraphics[width=0.8\textwidth]{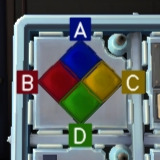}};
    \end{tikzpicture}
    \caption{Simon Says}
    \label{fig:simon_som}
\end{subfigure}%
\begin{subfigure}[t]{0.2\textwidth}
    \centering
    \begin{tikzpicture}
        \clip [rounded corners=5pt] (0,0) rectangle (0.8\textwidth, 0.8\textwidth);
        \node[anchor=south west, inner sep=0] at (0,0)
            {\includegraphics[width=0.8\textwidth]{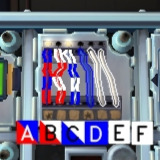}};
    \end{tikzpicture}
    \caption{Complicated\\Wires}
    \label{fig:comp-wires-som}
\end{subfigure}%
\begin{subfigure}[t]{0.2\textwidth}
    \centering
    \begin{tikzpicture}
        \clip [rounded corners=5pt] (0,0) rectangle (0.8\textwidth, 0.8\textwidth);
        \node[anchor=south west, inner sep=0] at (0,0)
            {\includegraphics[width=0.8\textwidth]{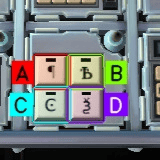}};
    \end{tikzpicture}
    \caption{Keypad}
    \label{fig:keypad-som}
\end{subfigure}%
\begin{subfigure}[t]{0.2\textwidth}
    \centering
    \begin{tikzpicture}
        \clip [rounded corners=5pt] (0,0) rectangle (0.8\textwidth, 0.8\textwidth);
        \node[anchor=south west, inner sep=0] at (0,0)
            {\includegraphics[width=0.8\textwidth]{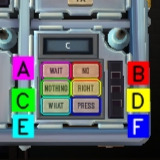}};
    \end{tikzpicture}
    \caption{Who's On First}
    \label{fig:whosonfirst-som}
\end{subfigure}
\caption{Examples of set-of-marks annotations applied to different bomb modules where colour is important to distinguish between elements.}
\label{fig:som-per-module-example}
\end{figure}
