# Supplementary material for: GPTNT: Benchmarking Real-Time Collaboration Between Multimodal Agents on Keep Talking And Nobody Explodes
Source: arXiv:2606.28514 source file (2026-09-04)
Supplement: Supplementary file 13 [file extended-reasoning.tex]

\paragraph{Extended reasoning exceeds practical time budgets.}
We explore using extended reasoning tokens---where models produce an internal chain-of-thought prior to any visible output \citep{DeepSeek-AI2025DeepSeekR1IncentivizingReasoning, OpenAI2024OpenAIO1System}---as a direct solution to the ordering problem identified with structured outputs. This is appealing as reasoning would always appear before the output.
Unfortunately, we find that models routinely consume more than 4,000 tokens (on average) before providing any visible output---this is consistent with documented tendencies for reasoning models to overthink problems without regulating token usage \citep{Su2025UnderthinkingOverthinkingEmpirical,Zhou2026WhenMoreThinking}.
Under typical throughput conditions, this translates to approximately one minute of wall-clock time per turn. This means that in the asynchronous mode, a single turn's reasoning budget consumes between one-third and one-fifth of the total time available, \textit{before} any action is taken.

\paragraph{Thinking budgets are not supported for all models.}
As we are using both open- and closed-source models, we want to control the thinking budget so that models think some, but not a lot. Unfortunately, the thinking budget or effort parameter is an API-level engineering knob and not a property of the underlying model. At the time of building, models served via vLLM did not have any support for these parameters. Since we do not want to diverge between open- and closed-source models, we opt to avoid using thinking entirely. For APIs where extended thinking cannot be fully disabled, the thinking budget is set to its minimum available value.\looseness=-1
