# Supplementary material for: GPTNT: Benchmarking Real-Time Collaboration Between Multimodal Agents on Keep Talking And Nobody Explodes
Source: arXiv:2606.28514 source file (2026-09-04)
Supplement: Supplementary file 14 [file nobf.tex]

\levelstay{Handling Parser Errors}\label{app:nobf}

While we provide the action schema in the system prompt, it is not enforced at the logit or API level. Given the cost of running experiments at scale, we prioritise salvaging imperfect outputs over discarding them.
We apply partial matching and fuzzy JSON recovery as fallback strategies before any feedback is triggered; minor deviations that can be resolved automatically produce no error signal at all.

When a malformed output cannot be silently recovered, feedback is provided via an
\texttt{<execution-feedback>} block prepended to that model's \textit{next} turn input. Errors fall into two tiers based on whether the intended action can proceed.

\paragraph{Soft warnings.}
When an action can be extracted despite structural imperfections in the output, the action proceeds and feedback is delivered on the following turn.
Conditions that trigger a soft warning include: the absence of a \texttt{<thoughts>} block; an action appearing before the closing \texttt{</thoughts>} tag; content appearing after \texttt{</action>}; and malformed XML structure, in which case the system first attempts JSON extraction from the raw output before flagging the structural issue separately.
Token budget violations are handled by the same salvage logic as other
malformed outputs: the truncated content is always returned to the model in
context regardless of outcome. If an action is recoverable from the truncated
output, the turn proceeds and the model is informed accordingly; if not, the
violation escalates to an unsalvageable error.

\paragraph{Unsalvageable errors.}
When no valid action can be recovered, the turn is skipped and the action is
blocked (and replaced with a \texttt{do\_nothing}).
These errors divide into two sub-cases.
\textit{Structural failures} occur when no coherent response can be extracted at all: no action is present in the output, multiple actions appear within a single turn, the output is wholly unparseable, or no action can be recovered from a token-budget-truncated response (in which case the truncated content is still returned to the model in context).
\textit{Semantic failures} occur when the output is well-formed but specifies an action that cannot be executed: an SoM label absent from the current annotation set, or coordinate values that fall outside screen bounds. In both sub-cases the model is informed that its previous turn was skipped and why, but no information about the broader game state or the consequences of any prior actions is conveyed.

\paragraph{Feedback mechanism.}
Feedback is always delivered on the model's \textit{next} scheduled turn rather than via an immediate retry, and the two are not equivalent.
By the time feedback arrives, the model receives it alongside fresh visual observations of the current game state, meaning it must re-perceive the environment before responding.
This is especially important in the asynchronous mode as game time continues to advance between the malformed turn and the subsequent one; therefore, feedback is always framed in terms of the \textit{previous} turn.
No retry is ever issued. While a retry is technically feasible in the synchronous mode since the clock has not advanced, we apply a no-retry policy across both modes to keep turn-level policy consistent across all experimental conditions.

The language of feedback messages has to reflect this structure. Directive phrasings---whether imperative (\textit{``produce a valid action''}) or softer (\textit{``you should check that your output is valid''})---cause models to treat feedback as a retry instruction, attempting the same action again on the new turn rather than re-engaging with the now-current game state.
This directly undermines the mechanism: delivering feedback alongside fresh observations is intended to force forward re-computation, and directive language pulls the model's attention back to the failed turn instead.
Past-tense, descriptive framing consistently avoids this. For example: \textit{``The response you generated caused you to skip your previous turn. Make sure to include an action in your response.''}
Framing feedback this way closes the door on the previous turn without prescribing behaviour on the current one, leaving the model to re-engage with its context rather than attempt a stale retry.
