# Supplementary material for: GPTNT: Benchmarking Real-Time Collaboration Between Multimodal Agents on Keep Talking And Nobody Explodes
Source: arXiv:2606.28514 source file (2026-09-04)
Supplement: Supplementary file 15 [file tool_calling.tex]

\paragraph{Tool calling requires a successful return.}
A core design decision in our setup is that models should not receive explicit feedback about the consequences of their actions. If a model performs an incorrect action that triggers a strike, it should infer what happened from subsequent visual observations alone, mirroring the standard assumption that an agent perceives the consequences of its actions rather than being told about them.
Tool calling is fundamentally at odds with this design. The API contract for tool calling requires that every tool invocation be followed by a corresponding tool return message \citep{Anthropic2026HowToolUse,OpenAI2026FunctionCalling}.\footnote{OpenAI asks that if your tool returns nothing, you return a string that simply indicates success or failure \citep{OpenAI2026FunctionCalling}.}
This forced incompatibility means that we have to provide \textit{some} return to the model after every action.

In early experiments, Pydantic AI supplied a generic string when using tools without returns---\texttt{``Final response processed.''}
Although this is semantically vacuous, we observe that models consistently interpret this as positive confirmation that their action has succeeded. Unfortunately, the consequences of this are severe: after an incorrect action that triggers a strike, a model using tool calling often hallucinates that a green LED exists and concludes that the module has been solved. Interestingly, this behaviour suggests a disconnect between how models reason over the different modalities.
The Defuser then sends congratulatory messages to the Expert, and both agents proceed to spend
several turns affirming that the task has been solved and that they have done well---all
while the bomb timer continues to count down.
As this happened repeatedly, we conclude that tool calling---in this form---is not suited to our domain.

\paragraph{Preserving a uniform interface.}
Models that have undergone tool-calling-specific fine-tuning carry an inherent format advantage: their training has optimised them for exactly this interaction pattern, independent of any collaborative or reasoning capabilities. Therefore, adopting a plain JSON interface ensures that all models---fine-tuned or otherwise---are evaluated on equal footing, and that any observed differences in performance reflect the collaborative capabilities.
