# Supplementary material for: GPTNT: Benchmarking Real-Time Collaboration Between Multimodal Agents on Keep Talking And Nobody Explodes
Source: arXiv:2606.28514 source file (2026-09-04)
Supplement: Supplementary file 16 [file message.tex]

\levelstay{Send Message}\label{app:action_space:send_message}

The \texttt{send\_message} action sends a free-form text string to the other player and is the sole method through which Defuser and Expert
can communicate:

\vspace{-15pt}
\begin{minted}[frame=lines,framesep=10pt,ignorelexererrors=true]{json}
{
  "result": {
    "kind": "send_message",
    "data": {
      "message": "Six wires: red, red, blue, yellow, black, white. Serial number ends in an odd digit."
    }
  }
}
\end{minted}
\vspace{-10pt}

Messages enter the recipient's pull queue immediately and are delivered atomically at the start of their next forward pass.
No message is ever dropped, summarised, or withheld---if the Defuser completes three turns during a long Expert generation, all three messages arrive together on the Expert's next turn.

Message content is also unconstrained in format and length, thereby allowing models to send full
observations, partial updates, questions, or multi-step instructions across consecutive
turns. They are only limited by the 1,000-token limit per model output.
