# Supplementary material for: GPTNT: Benchmarking Real-Time Collaboration Between Multimodal Agents on Keep Talking And Nobody Explodes
Source: arXiv:2606.28514 source file (2026-09-04)
Supplement: Supplementary file 17 [file expert-ocr-without-text.tex]

\levelstay{Ablation on Providing Text with Manual Input }
\label{app:expert-ocr-without-text}

In this work, we provide the manual to models using interleaved images and text. In \cref{tab:expert-ocr-text-comparison}, we compare how models perform on the Manual VQA Reading task (\cref{sec:statics:manual-vqa}) when we do not provide the text.
On average, models perform better by 4.3\% when additionally providing text for the manual.
GPT is the only exception, performing equally well in both conditions.

\begin{table}[tbh]
\centering
\footnotesize

\caption{Accuracy (\%) on Manual VQA Reading task by model, with and without the manual text provided.}
\label{tab:expert-ocr-text-comparison}
\begin{threeparttable}

\begin{tabular}{@{}l S[table-format=2.1] S[table-format=2.1] @{}}

\toprule
 & {Images + text} & {Images only} \\
\midrule
\claude*~Sonnet 4.6 & \Uline{75.9} & 71.2 \\
\gemini*~Gemini 3 Flash & \Uline{81.2} & 80.6 \\
\openai*~GPT-5.2 & \Uline{65.4} & \Uline{65.4}\\
\internvl*~InternVL 3.5 (38B) & \Uline{29.3} & 19.4 \\
\qwen*~Qwen3.5 (27B) & \Uline{68.6} & 62.3 \\
\midrule[0.1ex]
\textit{Average} & \Uline{64.1} & 59.8 \\
\bottomrule
\end{tabular}
\end{threeparttable}
\end{table}
