# Supplementary material for: GPTNT: Benchmarking Real-Time Collaboration Between Multimodal Agents on Keep Talking And Nobody Explodes
Source: arXiv:2606.28514 source file (2026-09-04)
Supplement: Supplementary file 18 [file table_async_single_module_self_play_outcomes.tex]

\begin{table}[tbh]
\centering
\footnotesize

\begin{threeparttable}
\caption{Self-play game outcomes across single-module missions in \textit{asynchronous} mode,
where the game clock \textit{runs continuously} during model generation. We examine mission
completion, strike distribution at timeout, and strikeout timing. Each model attempts
each single-module mission once (pass@1).}
\label{tab:async-single-module-self-play-outcomes}
\setlength{\tabcolsep}{4pt}
\sisetup{table-format=2.1}
\begin{tabular}{@{}l S S[table-format=3.1] S S S S S @{}}
\toprule
 & {\success* Solved} & \multicolumn{4}{c}{\timeout* Timeout} & \multicolumn{2}{c}{\strikeout* Strikeout} \\
\cmidrule(lr){2-2}\cmidrule(lr){3-6}\cmidrule(lr){7-8}
 & {\makecell{\% of\\Missions}}
 & {\makecell{\% of\\Failures}}
 & {0 Strikes}
 & {1 Strike}
 & {2 Strikes}
 & {\makecell{\% of\\Failures}}
 & {\makecell{Time\\Elapsed (\%)}} \\
\midrule
\claude*~Sonnet 4.6           & 12.7 & 84.4 & 50.6 & 32.1 & 17.3 & 15.6 & 71.9 \\
\gemini*~Gemini 3 Flash       & 14.5 & 88.3 & 85.5 & 9.6  & 4.8  & 11.7 & 53.6 \\
\openai*~GPT-5.2              & 8.2  & 92.1 & 65.6 & 24.7 & 9.7  & 7.9  & 79.9 \\
\internvl*~InternVL 3.5 (38B) & 4.5  & 64.8 & 51.5 & 27.9 & 20.6 & 35.2 & 44.8 \\
\qwen*~Qwen3.5 (27B)          & 7.3  & 91.2 & 64.5 & 23.7 & 11.8 & 8.8  & 57.6 \\
\midrule
\textit{Average}              & 9.5  & 84.1 & 63.5 & 23.6 & 12.8 & 15.9 & 61.6 \\
\bottomrule
\end{tabular}
\end{threeparttable}
\end{table}
