# Supplementary material for: GPTNT: Benchmarking Real-Time Collaboration Between Multimodal Agents on Keep Talking And Nobody Explodes
Source: arXiv:2606.28514 source file (2026-09-04)
Supplement: Supplementary file 19 [file table_sync_single_module_self_play_outcomes.tex]

\begin{table}[tbh]
\centering
\footnotesize

\begin{threeparttable}
\caption{Self-play game outcomes across single-module missions in \textit{synchronous} mode,
where the game clock \textit{pauses} while models generate. We examine mission completion,
strike distribution at timeout, and strikeout timing. Each model attempts each
single-module mission once (pass@1).}
\label{tab:sync-single-module-self-play-outcomes}
\setlength{\tabcolsep}{4pt}
\sisetup{table-format=2.1}
\begin{tabular}{@{}l S S S S S S S @{}}
\toprule
 & {\success* Solved} & \multicolumn{4}{c}{\timeout* Timeout} & \multicolumn{2}{c}{\strikeout* Strikeout} \\
\cmidrule(lr){2-2}\cmidrule(lr){3-6}\cmidrule(lr){7-8}
 & {\makecell{\% of\\Missions}}
 & {\makecell{\% of\\Failures}}
 & {0 Strikes}
 & {1 Strike}
 & {2 Strikes}
 & {\makecell{\% of\\Failures}}
 & {\makecell{Time\\Elapsed (\%)}} \\
\midrule
\claude*~Sonnet 4.6           & 39.1 & 31.3 & 52.4 & 23.8 & 23.8 & 68.7 & 59.2 \\
\gemini*~Gemini 3 Flash       & 20.9 & 64.4 & 80.4 & 5.4  & 14.3 & 35.6 & 49.6 \\
\openai*~GPT-5.2              & 38.2 & 54.4 & 32.4 & 32.4 & 35.1 & 45.6 & 50.9 \\
\internvl*~InternVL 3.5 (38B) & 12.7 & 59.4 & 68.4 & 19.3 & 12.3 & 40.6 & 44.0 \\
\qwen*~Qwen3.5 (27B)          & 10.9 & 77.6 & 65.8 & 23.7 & 10.5 & 22.4 & 55.2 \\
\midrule
\textit{Average}              & 24.4 & 57.4 & 59.9 & 20.9 & 19.2 & 42.6 & 51.8 \\
\bottomrule
\end{tabular}
\end{threeparttable}
\end{table}
