# Supplementary material for: GPTNT: Benchmarking Real-Time Collaboration Between Multimodal Agents on Keep Talking And Nobody Explodes
Source: arXiv:2606.28514 source file (2026-09-04)
Supplement: Supplementary file 20 [file context_management.tex]

\levelstay{Observation Context Management}

Accumulating visual observations across every turn causes the context to grow in direct proportion to game duration, and for models with smaller context windows this becomes a genuine problem — unconstrained image accumulation would rapidly exhaust available capacity, eventually displacing both the dialogue history and the manual. To handle this, each forward pass receives only the current turn's observation, one frame for standard modules or sixteen for \morsecode and \simonsays, along with a single unannotated frame from the immediately preceding turn, with everything older discarded.

That previous frame turns out to matter quite a bit. Without it there's no reliable way to tell whether the last action produces any visible change---a correctly placed click changes the game state in ways that are easy to see, while a mis-click on a neutral region leaves everything exactly as it is.
Keeping that one prior frame makes the consequence of the preceding action directly observable, at the cost of a single additional image per turn.\looseness=-1
