# Supplementary material for: GPTNT: Benchmarking Real-Time Collaboration Between Multimodal Agents on Keep Talking And Nobody Explodes
Source: arXiv:2606.28514 source file (2026-09-04)
Supplement: Supplementary file 21 [file how_many_images_from_buffer.tex]

\levelstay{Temporal Observations}

For most modules---where reading the current state means nothing more than a single snapshot---only the most recent frame (and preceding frame) is passed to the Defuser on each forward pass. However, modules like \morsecode and \simonsays are exceptions: both encode information in blinking light sequences that unfold over time and simply cannot be decoded from any individual frame, so for these the full sixteen-frame buffer from the mod (\cref{app:mod:frames}) is transmitted to models.
That depth of sixteen is empirically verified to contain at least one complete blink cycle for both modules---for Morse, one cycle corresponds to the longest letter. Transmitting full video sequences is considered as an alternative but rejected on token cost grounds.

Despite our best efforts, models can occasionally miss a complete sequence within a single window, usually because the observation lands poorly timed relative to the blink period. The correct response is to emit a \texttt{do\_nothing} action and re-observe on the following turn, which mirrors what human players do under the same circumstances.
