# Supplementary material for: GPTNT: Benchmarking Real-Time Collaboration Between Multimodal Agents on Keep Talking And Nobody Explodes
Source: arXiv:2606.28514 source file (2026-09-04)
Supplement: Supplementary file 22 [file observations.tex]

\levelstay{Observations}\label{app:observations}

While we do export a JSON representation of the environment, we never provide this to models because this would make the task too easy. Models must use the modalities available to them---just like a human player---to solve the task. We strongly recommend against adapting the benchmark to provide this information to models because the complexity stemming from the visual observations would be muted, resulting in a drastically simplified task.\looseness=-1

\subimportlevel{observation}{resolution}{1}
\subimportlevel{observation}{set-of-marks}{1}
\subimportlevel{observation}{how_many_images_from_buffer}{1}
\subimportlevel{observation}{context_management}{1}
