# Supplementary material for: GPTNT: Benchmarking Real-Time Collaboration Between Multimodal Agents on Keep Talking And Nobody Explodes
Source: arXiv:2606.28514 source file (2026-09-04)
Supplement: Supplementary file 23 [file output_format.tex]

\levelstay{Output Format}\label{app:output-format}

As Transformer-based models generate tokens autoregressively, only content generated before an action token can mechanistically influence that action. Content generated after is a post-hoc rationalisation rather than deliberation, as it cannot retroactively alter the committed output.
The chain-of-thought literature establishes that eliciting explicit intermediate reasoning prior to the final response reliably improves model performance by using this causal structure \citep{Wei2022ChainofThoughtPromptingElicits}. ReAct \citep{Yao2022ReActSynergizingReasoning} extends this principle to interactive, action-taking settings, enabling models to use reasoning traces to ground each decision in explicit thought before it is committed.
This therefore yields a non-negotiable requirement for the output format: the reasoning trace must precede the action in the model output.

\subimportlevel{output_format}{react_xml}{1}
\subimportlevel{output_format}{nobf}{1}

\leveldown{Alternatives Considered}

\subimportlevel{output_format}{tool_calling}{1}
\subimportlevel{output_format}{structured_outputs}{1}
\subimportlevel{output_format}{extended-reasoning}{1}
