# Supplementary material for: GPTNT: Benchmarking Real-Time Collaboration Between Multimodal Agents on Keep Talking And Nobody Explodes
Source: arXiv:2606.28514 source file (2026-09-04)
Supplement: Supplementary file 24 [file react_xml.tex]

\levelstay{XML-delimited ReAct}

All models must provide their output following a custom XML-tag-based ReAct formulation:
\begin{minted}{xml}
<thoughts>
    [free-form text - no schema constraints]
</thoughts>
<action>
    {"result": {"kind": "...", "data": {...}}}
</action>
\end{minted}

The \texttt{<thoughts>} block accepts arbitrary free-form text with no length or content constraints; models can choose to abstain from providing thoughts too. The tag name \texttt{<thoughts>} is chosen deliberately as it is semantically neutral across all five models evaluated, carrying no pre-existing association with any specialised inference mode.

The \texttt{<action>} block contains the action JSON as specified in \cref{app:action_space}.
XML delimiters enforce the required ordering at the structural level: a model should not emit an action until the thoughts block has been closed.
In practice, we find that this method is reliable as models that produce any reasoning at all place it before the action.
