# Supplementary material for: GPTNT: Benchmarking Real-Time Collaboration Between Multimodal Agents on Keep Talking And Nobody Explodes
Source: arXiv:2606.28514 source file (2026-09-04)
Supplement: Supplementary file 25 [file structured_outputs.tex]

\paragraph{Structured outputs cannot enforce field ordering.}
Structured outputs (e.g., \citealp{Dong2025XGrammarFlexibleEfficient}) are an obvious mechanism for enforcing well-formed responses, but JSON schemas have no means of constraining the order in which fields are outputted.
As mentioned above, we want to ensure that models reason before acting, and a way to do this---without using extended reasoning---is to provide it as an optional field within the output JSON. However, there is no way to guarantee that a \texttt{thoughts} field precedes the action. In practice, we often see models committing to the action first, and providing the thoughts afterwards as a post-hoc justification.\looseness=-1
