# Supplementary material for: GPTNT: Benchmarking Real-Time Collaboration Between Multimodal Agents on Keep Talking And Nobody Explodes
Source: arXiv:2606.28514 source file (2026-09-04)
Supplement: Supplementary file 26 [file som-creation.tex]

\begin{figure}[tb]
\centering
\begin{subfigure}[t]{0.30\textwidth}
    \centering
    \begin{tikzpicture}
    \clip [rounded corners=5pt] (0,0) rectangle (1\textwidth, 1\textwidth);
    \node[anchor=south west, inner sep=0] at (0,0)
        {\includegraphics[width=1\textwidth]{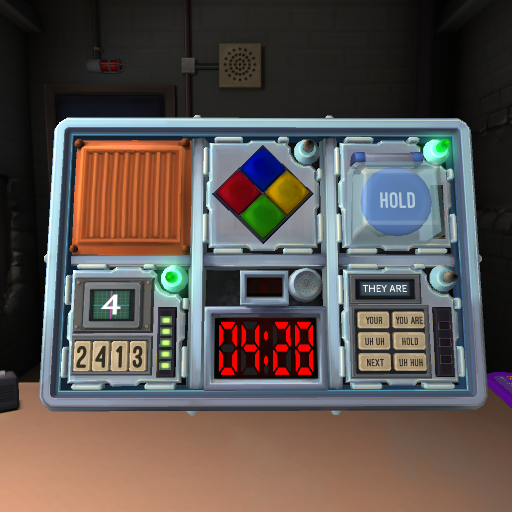}};
    \end{tikzpicture}
    \caption{Original frame}
    \label{fig:som-original}
\end{subfigure}%
\hspace{\fill}
\begin{subfigure}[t]{0.30\textwidth}
    \centering
    \begin{tikzpicture}
    \clip [rounded corners=5pt] (0,0) rectangle (1\textwidth, 1\textwidth);
    \node[anchor=south west, inner sep=0] at (0,0)
        {\includegraphics[width=1\textwidth]{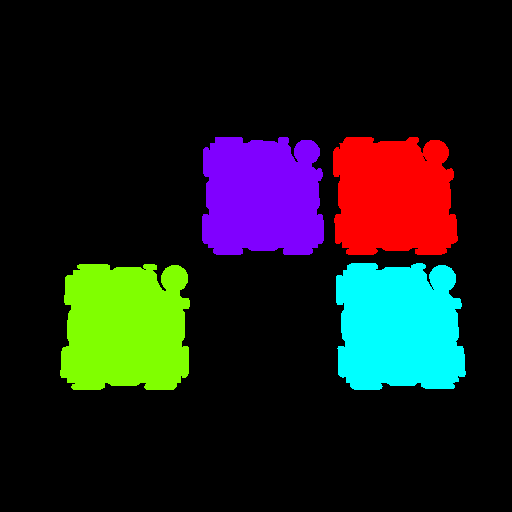}};
    \end{tikzpicture}
    \caption{Segmentation mask}
    \label{fig:som-segm-mask}
\end{subfigure}%
\hspace{\fill}
\begin{subfigure}[t]{0.30\textwidth}
    \centering
    \begin{tikzpicture}
    \clip [rounded corners=5pt] (0,0) rectangle (1\textwidth, 1\textwidth);
    \node[anchor=south west, inner sep=0] at (0,0)
        {\includegraphics[width=1\textwidth]{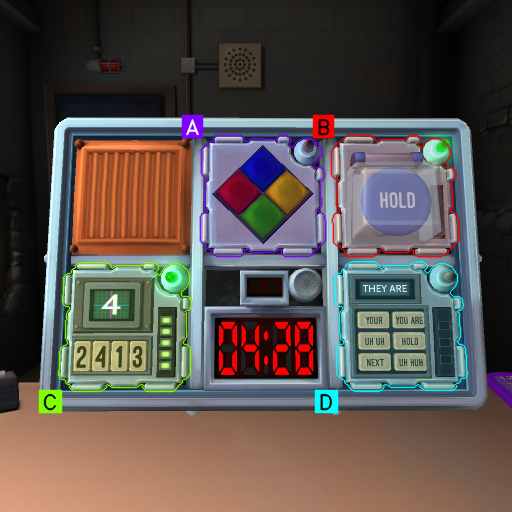}};
    \end{tikzpicture}
    \caption{Image with annotations}
    \label{fig:som-final}
\end{subfigure}%
\caption{Set-of-Marks annotation inputs and outputs. The original frame (a) and segmentation mask (b) are both provided by the environment using our mod. In the segmentation mask, each interactable object is represented by a distinct colour region. Using a heuristic pipeline, we generate the annotated image (c) which combines the previous two images and provide that to the model to facilitate easier identification of interactable elements.}
\label{fig:som-creation}
\end{figure}
