# Supplementary material for: GPTNT: Benchmarking Real-Time Collaboration Between Multimodal Agents on Keep Talking And Nobody Explodes
Source: arXiv:2606.28514 source file (2026-09-04)
Supplement: Supplementary file 27 [file som-per-module-examples.tex]

\begin{figure}[htb]
\centering
\begin{subfigure}[t]{0.2\textwidth}
    \centering
    \begin{tikzpicture}
        \clip [rounded corners=5pt] (0,0) rectangle (0.8\textwidth, 0.8\textwidth);
        \node[anchor=south west, inner sep=0] at (0,0)
            {\includegraphics[width=0.8\textwidth]{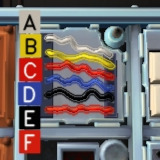}};
    \end{tikzpicture}
    \caption{Wires}
    \label{fig:sub-wires}
\end{subfigure}%
\begin{subfigure}[t]{0.2\textwidth}
    \centering
    \begin{tikzpicture}
        \clip [rounded corners=5pt] (0,0) rectangle (0.8\textwidth, 0.8\textwidth);
        \node[anchor=south west, inner sep=0] at (0,0)
            {\includegraphics[width=0.8\textwidth]{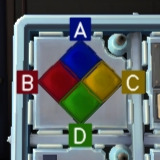}};
    \end{tikzpicture}
    \caption{Simon Says}
    \label{fig:simon_som}
\end{subfigure}%
\begin{subfigure}[t]{0.2\textwidth}
    \centering
    \begin{tikzpicture}
        \clip [rounded corners=5pt] (0,0) rectangle (0.8\textwidth, 0.8\textwidth);
        \node[anchor=south west, inner sep=0] at (0,0)
            {\includegraphics[width=0.8\textwidth]{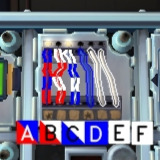}};
    \end{tikzpicture}
    \caption{Complicated\\Wires}
    \label{fig:comp-wires-som}
\end{subfigure}%
\begin{subfigure}[t]{0.2\textwidth}
    \centering
    \begin{tikzpicture}
        \clip [rounded corners=5pt] (0,0) rectangle (0.8\textwidth, 0.8\textwidth);
        \node[anchor=south west, inner sep=0] at (0,0)
            {\includegraphics[width=0.8\textwidth]{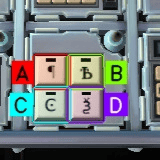}};
    \end{tikzpicture}
    \caption{Keypad}
    \label{fig:keypad-som}
\end{subfigure}%
\begin{subfigure}[t]{0.2\textwidth}
    \centering
    \begin{tikzpicture}
        \clip [rounded corners=5pt] (0,0) rectangle (0.8\textwidth, 0.8\textwidth);
        \node[anchor=south west, inner sep=0] at (0,0)
            {\includegraphics[width=0.8\textwidth]{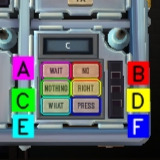}};
    \end{tikzpicture}
    \caption{Who's On First}
    \label{fig:whosonfirst-som}
\end{subfigure}
\caption{Examples of set-of-marks annotations applied to different bomb modules where colour is important to distinguish between elements.}
\label{fig:som-per-module-example}
\end{figure}
